# Supplementary material for: MagicVL-2B: Empowering Vision-Language Models on Mobile Devices with Lightweight Visual Encoders via Curriculum Learning
Source: arXiv:2508.01540 source file (2025-08-03)
Supplement: Supplementary file 1 [file 6_appendix.tex]

\section{Appendix}

\subsection{Examples of Data Cleaning}
A primary objective of our data cleaning pipeline is to remove samples containing repetitive textual content. As illustrated in Figure~\ref{fig:repetitionexamples}, repetitive generation is a prevalent issue in large-scale datasets, particularly those that are artificially synthesized. The adoption of our rule-based filtering system resulted in a substantial reduction in the frequency of anomalous model behaviors, most notably repetitive output generation. Furthermore, this data cleaning pipeline led to significant improvements in the model's performance across a variety of tasks, demonstrating its effectiveness in fostering more robust and reliable model behavior in diverse evaluation scenarios.
\begin{figure*}[htbp]
    \centering
    \begin{subfigure}[t]{0.45\textwidth}
        \centering
        \includegraphics[width=\textwidth]{figure/data_example1.png}
        \caption{\textbf{Question}: Give a detailed account of this image.\\ \textbf{Answer}: Screenshot that says segment, the, are, cust, product, pricing, docs, company, login, sign up, marketing, product, engineering, connections, protocols, personas, functions, warehouses, privacy, GDPR, catalog, use cases. The background is mostly gray, but there's white in the center. The outer background is like a darker blue. The background is mostly gray, but there's white in the center. \textcolor{red}{The background is mostly gray, but there's a lot of text. The background is mostly gray, but there's a lot of text. The background is mostly gray, but there's a lot of text.}}
        \label{fig:repetitionexample1}
    \end{subfigure}
    \hspace{0.05\textwidth}
    \begin{subfigure}[t]{0.45\textwidth}
        \centering
        \includegraphics[width=\textwidth]{figure/data_example2.jpeg}
        \caption{\textbf{Question}: Give a short and clear explanation of the subsequent image. \\ \textbf{Answer}: Crispy, black background, then there are \textcolor{red}{dots, dots, dots, dots, dots, dots, dots, dots.} And there is yellow, it says old, parenthesis 6.3.24. The quick brown fox jumps over the lazy dog, I think it's font, so it's some kind of cursive font, gray, then there's a line, it's gray, it says the quick brown fox jumps over the lazy dog, the dot, and new, the text is 6.3.33, and so there are a lot of dots, dots, dots, dots, dots, and yeah, quick brown fox jumps over lazy dog, quick brown fox jumps over lazy dog, slightly updated font, a little thinner, and they're more distinct, the letters. And perhaps this is someone's advertisement for this one?}
        \label{fig:repetitionexample2}
    \end{subfigure}
    \caption{Data examples that have repetitive patterns. Dataset source: PixMo~\cite{deitke2024molmo}}
    \label{fig:repetitionexamples}
\end{figure*}

\begin{table*}[htbp]
\centering
\begin{tabular}{|c|p{14cm}|}
\hline
\textbf{Task} & \textbf{Datasets} \\
\hline
General & InfinityMM~\cite{gu2024infinity}, ALLaVA~\cite{chen2024allava}, Cambrian-10M~\cite{tong2024cambrian1}, PixMo~\cite{deitke2024molmo}, Llava-OneVision~\cite{li2024llava} \\
\hline
Caption & ShareGPT4V~\cite{chen2024sharegpt4v}, ShareGPT4o~\cite{cui2025comprehensive}, Llava558k~\cite{liu2023improvedllava}, MMC-Alignment~\cite{liu2023mmc}, LLaVA-CC3M-Pretrain-595K~\cite{liu2023improvedllava} \\
\hline
OCR & DocDownstream~\cite{ye2023mplug}, DocReason~\cite{ye2023mplugowl}, DocStruct~\cite{ye2023mplugowl}, Cocotext~\cite{veit2016coco}, DocVQA~\cite{mathew2021docvqa}, ST-VQA~\cite{biten2019scene}, Docmatix~\cite{laurençon2024building}, Ocr-vqa~\cite{mishra2019ocrvqa}, SynthDog~\cite{kim2021donut},  WIkiSQL~\cite{zhong2017seq2sql}, IconQA~\cite{lu2021iconqa}\\
\hline
Chart & ChartQA~\cite{masry2022chartqa}, MMC-Inst~\cite{liu2023mmc}, DVQA~\cite{kafle2018dvqa}, ArxivQA~\cite{li2024multimodal}, Chart2Text~\cite{kantharaj2022chart}, FigureQA~\cite{kahou2017figureqa}, PlotQA~\cite{methani2020plotqa}, AI2D~\cite{kembhavi2016diagram}, FinQA~\cite{chen2021finqa},  InfoVQA~\cite{mathew2022infographicvqa}\\
\hline
VQA & LVIS-Instruct4V~\cite{wang2023instruct4v},  SketchyVQA~\cite{tu2023many}, OODVQA~\cite{tu2023many}, VizWiz~\cite{gurari2018vizwiz}, Q-Instruct~\cite{wu2024q}, VisDial~\cite{das2017visual}, Llava665k~\cite{liu2023improvedllava},  LAION GPT-4V~\cite{laion2023gpt4v}, AlfWorld~\cite{shridhar2020alfworld}, LNQA~\cite{pont2020connecting}, OKVQA~\cite{marino2019ok},  A-OKVQA~\cite{schwenk2022okvqa} \\
\hline
Reasoning & CLEVR~\cite{johnson2017clevr}, Super-CLEVR~\cite{li2023super}, TallyQA~\cite{acharya2019tallyqa}, Visualmrc~\cite{tanaka2021visualmrc}, GQA~\cite{hudson2019gqa}, VisualGenome~\cite{krishna2017visual}, RAVEN~\cite{zhang2019raven}, MathQA~\cite{amini2019mathqa}, MathV360k~\cite{shi2024math}, Geo170K~\cite{gao2023g}, ScienceQA~\cite{lu2022learn}, HatefulMemes~\cite{kiela2020hateful},   \\
\hline
GUI & Screen2Words~\cite{wang2021screen2words}, WebSight~\cite{laurenccon2024unlocking}, Design2Code~\cite{si2403design2code}, AndroidControl~\cite{li2024effects}, AITW~\cite{rawles2023androidinthewild}, GUI-Odyssey~\cite{lu2024gui}\\
\hline
Text & SmolTalk~\cite{allal2025smollm2smolgoesbig}, Dolly~\cite{conover2023free},  MathInstruct~\cite{yue2023mammoth}, WizardCoder~\cite{luo2023wizardcoder}, OrcaMath~\cite{mitra2024orca}, Open-CodeInterpreter~\cite{zheng2024opencodeinterpreter}, OpenOrca~\cite{lian2023openorca}, Infinity-Instruct~\cite{li2025infinity} \\
\hline
\end{tabular}
\caption{Summary of the training data collection of MagicVL}
\end{table*}

\subsection{Optimal Weight Calibration via Human-Annotated Difficulty Alignment}
To determine the optimal values for the weights $\{\lambda_i\}_{i=1}^{3}$ for each data category, we adopted a data-driven approach grounded in human annotation. For each data category, we curated five subsets from open-source datasets, each representing a distinct level of difficulty. For each difficulty level, we randomly sampled and manually annotated 1,000 data points, resulting in five datasets with increasing difficulty, as assessed by human experts. For each subset, we calculated the difficulty score $S$ as previously defined using various candidate values of $\{\lambda_i\}_{i=1}^{3}$. The objective was to select weights such that the resulting $S$ scores for the five constructed datasets strictly reflected the intended ordering of difficulty. We performed a grid search over feasible values of $\{\lambda_i\}_{i=1}^{3}$ and selected the set of weights that maximized the monotonic alignment between the computed $S$ scores and the expert-annotated difficulty levels. In addition, we ensured that the margin between $S$ scores of consecutive difficulty levels was sufficiently large to guarantee robust differentiation.

\subsection{Examples of Data at Different Levels of Difficulty}

To qualitatively validate the effectiveness of our difficulty-level annotation framework, Figure~\ref{fig:difficulty_examples} presents representative VQA data samples corresponding to different difficulty levels. Specifically, the example on the left illustrates a data sample categorized as easy, while the example on the right represents a hard data sample.

% from each difficulty level within our dataset. As illustrated, the "very easy" example contains a clear and straightforward visual scene and question, resulting in similar and low loss values across all model sizes. In the "easy" example, a higher degree of contextual reasoning is required, leading to more noticeable differences in loss values, especially for the 2B-sized model. For the "medium" and "hard" samples, the scenes become progressively more complex, necessitating abstract reasoning or the ability to count objects while handling occlusion. The loss values indicate that larger models tend to outperform smaller ones as the task difficulty increases.

\begin{figure*}[htbp]
    \centering
    \begin{tabular}{cc}
        \begin{subfigure}[b]{0.45\textwidth}
            \centering
            \includegraphics[width=\linewidth]{figure/example_easy.png}
            \caption{\textbf{Question}: What's the man doing? Answer the question using one word.\\ \textbf{Answer}: Riding \\ $M_{2B}=1.03 \quad M_{7B}=1.05 \quad M_{72B}=1.04$}
        \end{subfigure} &
        \begin{subfigure}[b]{0.45\textwidth}
            \centering
            \includegraphics[width=\linewidth]{figure/example_hard.png}
            \caption{\textbf{Question}: Context: The images below show two pairs of magnets. The magnets in different pairs do not affect each other. All the magnets shown are made of the same material.\\Question: Think about the magnetic force between the magnets in each pair. Which of the following statements is true?\\Options:\\A. The magnetic force is weaker in Pair 2.\\B. The magnetic force is weaker in Pair 1.\\C. The strength of the magnetic force is the same in both pairs.\\Answer the question by selecting only one option from the given options. Answer the question using one letter.\\ \textbf{Answer}: B \\ $M_{2B} = 0.98 \quad M_{7B}=0.51 \quad M_{72B}=0.01$}
        \end{subfigure}
    \end{tabular}
    \caption{Examples of data at different levels of difficulty.}
    \label{fig:difficulty_examples}
\end{figure*}

\begin{figure*}[htbp]
\centering
\includegraphics[width=\textwidth]{figure/dynamic.pdf}
\caption{
\textbf{Comparison of dynamic resolution processing strategies.}
(a) Raw image with original size $940 \times 479$.
(b) BlueLM-V-3B resizes the image to $1152 \times 384$, resulting in aspect ratio distortion.
(c) InternVL resizes the image to $1536 \times 768$, leading to significant enlargement and increased token count.
(d) MagicVL-2B pads the image to $960 \times 480$, effectively preserving the original content.
The check mark indicates the optimal solution for maintaining integrity of the input image.
}
\label{fig:dynamic_res_example}
\end{figure*}

\subsection{Examples of Different Dynamic Resolution Methods}

We illustrate the effects of different dynamic resolution methods on image processing. Figure~\ref{fig:dynamic_res_example} displays an example image with dimensions of 940$\times$479, where the length is significantly greater than the width. Both LLaVA and InternVL methods enlarge the image, resulting in a substantial increase in the number of tokens. BlueLM-V-3B~\cite{lu2024bluelm} approach distorts the image, which can adversely impact the recognition of fixed-pattern content. In contrast, our MagicVL-2B employs padding to match the encoder’s input size, thereby preserving the original image content and structure.

\begin{table*}[ht]
\resizebox{\textwidth}{!}{%
\begin{tabular}{lccccccc}
\midrule
\textbf{Visual Encoder} & \textbf{Input Size} & \textbf{Patch Size} & \textbf{Viusal Params} & \textbf{AI2D} & \textbf{OCRBench} & \textbf{ DocVQA} \\ \midrule
ViT-Base~\cite{ViT}      & 224 & 16 & 86M & 70.2 & 696 & 74.2 \\
SigLIP-2-Base~\cite{tschannen2025siglip} & 224 & 16 & 93M & 72.3 & 726 & 80.7 \\
SigLIP-2-Base~\cite{tschannen2025siglip} & 256 & 16 & 93M & 74.1 & 744 & 83.2 \\
SigLIP-2-Base~\cite{tschannen2025siglip} & 256 & 32 & 95M & 46.1 & 518 & 67.3 \\
\rowcolor{gray!20} SigLIP-2-Base~\cite{tschannen2025siglip} & 384 & 16 & 93M & \textbf{76.7} & \textbf{775} & \textbf{87.7} \\ \midrule

\end{tabular}
}
% \vspace{-0.7em}
\caption{\textbf{Ablation experiment results on visual encoders and hyperparameters.}}
\label{tab:ablation_ve}
% \vspace{-0.5em}
\end{table*}

\subsection{Ablation Experiments of the Visual Encoder}

We conducted a series of ablation studies to systematically evaluate the impact of different visual encoder architectures and hyperparameter settings, while keeping the LLM fixed as Qwen2.5. As shown in Table~\ref{tab:ablation_ve}, we compared ViT-Base and several configurations of SigLIP-2-Base, varying the input size and patch size. The results indicate that increasing the input size generally leads to improved performance across all benchmarks. In particular, the SigLIP-2-Base encoder with an input size of 384 and a patch size of 16 achieves the highest scores on A12D, OCRBench, and DocVQA, significantly outperforming both smaller input sizes and larger patch sizes. This demonstrates the effectiveness of larger input resolutions and finer patch granularity for visual understanding tasks.
